# Supplementary material for: Minimization of atomic displacements as a guiding principle of the martensitic phase transformation
Source: arXiv:1912.11915 ancillary file (2020-09-22)
Supplement: Supplementary file 1 [file supp.pdf]

# Supplementary Material

## SHORT DESCRIPTION OF THE ALGORITHM

Fig. 1 illustrates the method for a simple two-dimensional example; the general principle is the same for real systems. The first step is to cut large finite portions of both the initial and final crystal structures to obtain two sets of points. Then, the initial structure (in red) is randomly aligned with respect to the final structure (in gray). The optimal mapping (i.e., the correspondence between each atom) is then established for that position. Since the sum of distances between each pair of atoms is now well defined ($d_1$), it is minimized with respect to the position of the final structure (in red) while the atoms are simultaneously remapped. The random initial alignment and the distance minimization are repeated several times such that the global minimum can be found. Finally, once the minimal distance is found, the algorithm retrieves the periodicity in the corresponding optimal mapping to obtain $C^x$ and $\{\mathbf{p}_x(l) : l = 1 \ldots m\}$.

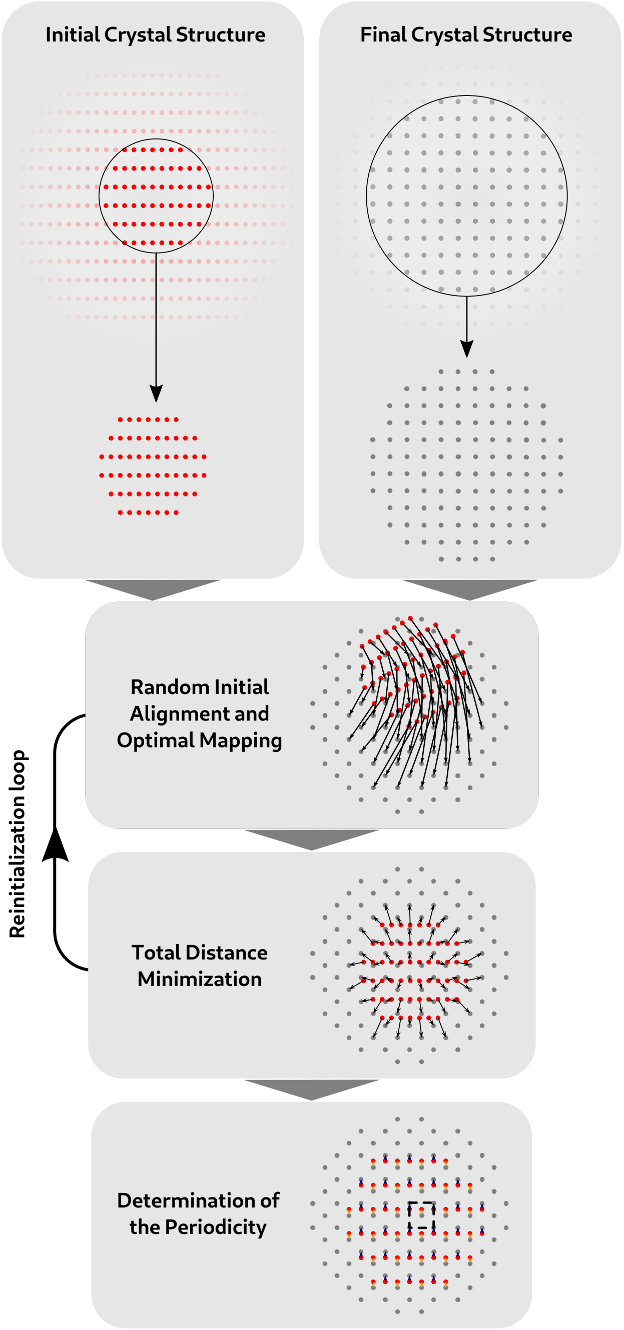


FIG. 1. Simplified visual representation of the behavior of the crystal structure matching algorithm.

The set of $C^x$ and $\{\mathbf{p}_x(l) : l = 1 \ldots m\}$ fully defines the mapping and correspond to a unique distance $d_1$. For example, in the Bain transformation, the FCC cell vectors ($C^\gamma$) would be $[110]a_\gamma/2$, $[1\bar{1}0]a_\gamma/2$ and $[100]a_\gamma$ where $a_\gamma$ is the austenite lattice constant. The martensite cell vectors would be that of the conventional BCC cell rotated clockwise by 45° about the c-axis. There would be one atom at the origin and one at the center of both cells (the relative atomic positions would not change during the transformation). This particular choice of the $C^x$ and $\{\mathbf{p}^x_l : l = 1 \ldots m\}$ for both structures fully describes the Bain transformation mechanism and it corresponds to a unique distance $d_1$ which, for the martensitic transformation, is not the minimal distance (the algorithm finds the mechanism presented in the paper instead).

Ignoring the periodicity at first by matching large finite portions of the crystals directly, atom-to-atom, avoids issues associated with matching the unit cells (see Fig. 2 in Ref. [1]). This is why the result presented in this paper cannot be obtained with our previous algorithm [2] which rely on such a procedure. A more detailed explanation of the method can be found in Ref. [1]. We wish to emphasize the fact that the algorithm requires only the lattice parameters of the initial and final structure; no other, information about the transformation is known a priori.

## EIGENVECTORS MATRICES

The following expression is the matrix $P$ whose columns are the eigenvectors of $U$ such that $U = P\,\mathrm{diag}(\lambda_1, \lambda_2, \lambda_3)\,P^T$. Its columns represent strain directions in the basis of austenite.

$$P = \begin{pmatrix} \frac{1}{\sqrt{2}} & \frac{1}{\sqrt{2}} & 0 \\ -\frac{1}{\sqrt{2}} & \frac{1}{\sqrt{2}} & 0 \\ 0 & 0 & 1 \end{pmatrix} \qquad (1)$$

Equivalently, the following expression is the matrix $Q$ whose columns are the eigenvectors of the strain matrix $V$

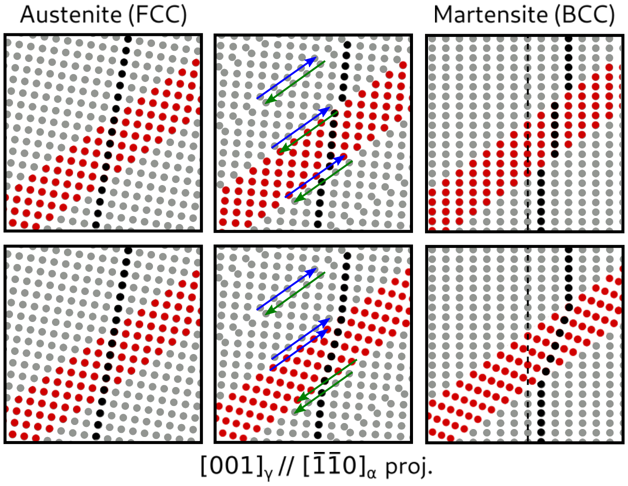


FIG. 2. Comparison of the slipping and twinning processes. The transformation is illustrated in 3 steps from left to right. Panels on the bottom row show the twinning process, where, in the red region, the displacements of the atoms have been inverted.

such that $V = Q\,\mathrm{diag}(1/\lambda_1, 1/\lambda_2, 1/\lambda_3)\,Q^T$. Its columns represent strain directions in the basis of martensite.

$$Q = \begin{pmatrix} \frac{1}{\sqrt{6}} & -\frac{1}{\sqrt{3}} & -\frac{1}{\sqrt{2}} \\ -\frac{1}{\sqrt{6}} & \frac{1}{\sqrt{3}} & -\frac{1}{\sqrt{2}} \\ \sqrt{\frac{2}{3}} & \frac{1}{\sqrt{3}} & 0 \end{pmatrix} \tag{2}$$

## OBTAINING A TWINNED LATTICE FROM THE OPTIMAL DISTANCE MECHANISM

Using the transformation cell of Fig.1 (article), one can construct an austenite crystal and transform it to martensite by applying the transformation matrix $T$ and the atomic displacements $\{\mathbf{t}_l = T^{-1}\mathbf{p}_l^{\alpha} - \mathbf{p}_l^{\gamma} : l = 1\ldots m\}$. This will always lead to a perfect BCC lattice since our algorithm found the optimal transformation mechanism between austenite and a perfect (untwined) martensite. However, Fig. 2 shows how twinned BCC can be obtained by inverting the direction $(-\mathbf{t}_l)$ of the local displacements of the atoms for one column of transformation cells along the $[110]\gamma||[\bar{1}11]_{\alpha}$ direction.

## COMPLETE STEPS TO OBTAIN THE UNIFORMLY SCALED PLANE

Vectors of the uniformly scaled plane obey the following equation:

$$||T\mathbf{u}|| = k||\mathbf{u}||\,, \tag{3}$$

where k is a scalar, independent of the choice of $\mathbf{u}$. We can write:

$$\mathbf{u}^T U^2 \mathbf{u} = k^2 \mathbf{u}^T \mathbf{u} \tag{4}$$

$$\mathbf{u}^T (U^2 - k^2 I)\mathbf{u} = 0 \tag{5}$$

$$\bar{\mathbf{u}}^T (D^2 - k^2 I)\bar{\mathbf{u}} = 0 \tag{6}$$

$$\bar{\mathbf{u}}^T \begin{pmatrix} {\lambda_1}^2 - k^2 & 0 & 0 \\ 0 & {\lambda_2}^2 - k^2 & 0 \\ 0 & 0 & {\lambda_3}^2 - k^2 \end{pmatrix} \bar{\mathbf{u}} = 0 \tag{7}$$

where $\bar{\mathbf{u}} = P^T\mathbf{u}$ are the vectors of the uniformly scaled plane expressed in terms of the principal strain directions (in the basis of the eigenvectors) and $\lambda_{1,2,3}$ are the eigenvalues of $U$ such that $\lambda_1 < \lambda_2 < \lambda_3$. This equation takes the form:

$$({\lambda_1}^2 - k^2){\bar{\mathbf{u}}_x}^2 + ({\lambda_2}^2 - k^2){\bar{\mathbf{u}}_y}^2 + ({\lambda_3}^2 - k^2){\bar{\mathbf{u}}_z}^2 = 0\,, \tag{8}$$

Equation (8) becomes the equation of a plane in 3D only if $k = \lambda_2$, in which case it becomes:

$$\bar{\mathbf{u}}_x \pm \sqrt{\frac{{\lambda_3}^2 - {\lambda_2}^2}{{\lambda_2}^2 - {\lambda_1}^2}}\,\bar{\mathbf{u}}_z = 0\,, \tag{9}$$

For example, with $\lambda_1 = \frac{2\sqrt{2}}{3}$, $\lambda_2 = 1$ and $\lambda_3 = \frac{2}{\sqrt{3}}$. We have:

$$\bar{\mathbf{u}}_x \pm \sqrt{3}\bar{\mathbf{u}}_z = 0\,. \tag{10}$$

. The vector $[\sqrt{2}\,0 \pm \sqrt{6}]$ is perpendicular to that plane and it can be expressed in coordinates of the austenite lattice:

$$\mathbf{n}_{\mathrm{HP}} = P\begin{pmatrix} \sqrt{2} \\ 0 \\ \pm\sqrt{6} \end{pmatrix} = \begin{pmatrix} 1 \\ -1 \\ \pm\sqrt{6} \end{pmatrix}. \tag{11}$$

## COMPLETE STEPS TO OBTAIN THE ROTATION MATRIX

The rotation $R$ is the one for which the invariant plane does not rotate during the transformation. This can be expressed mathematically as:

$$\frac{RU\mathbf{v}}{||RU\mathbf{v}||} = \mathbf{v}\,. \tag{12}$$

Where $\mathbf{v}$ are unitary vectors of the invariant plane. We have the following equations for two linearly independent vectors in the invariant plane:

$$R\frac{U\mathbf{v}_1}{||U\mathbf{v}_1||} = \mathbf{v}_1\,, \tag{13}$$

$$R\frac{U\mathbf{v}_2}{||U\mathbf{v}_2||} = \mathbf{v}_2\,, \tag{14}$$

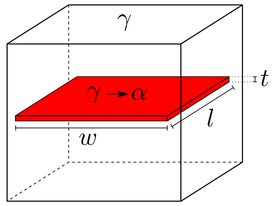


FIG. 3. Schematic of the plate. The atoms of the region in red undergo a martensitic transformation. The other atoms remain in their austenite initial state.

From these two, we can produce a third equation:

$$R\frac{(U\mathbf{v}_1 \times U\mathbf{v}_2)}{||U\mathbf{v}_1||||U\mathbf{v}_2||} = \mp\mathbf{n}^*_{\mathrm{HP}}\,. \tag{15}$$

Where $\mathbf{n}^*_{\mathrm{HP}}$ is the unitary vector normal to the invariant plane (equation (11)). Let us choose $v_1 = [\frac{1}{\sqrt{2}}\;\frac{1}{\sqrt{2}}\;0]$ and $v_2 = [\frac{\sqrt{6}}{4}\;-\frac{\sqrt{6}}{4}\;\mp\frac{1}{2}]$ such that they are orthogonal and unitary. We can rewrite equations (13), (14), and (15) in matrix form:

$$RM = V\,, \tag{16}$$

where

$$M = \left(\frac{U\mathbf{v}_1}{||U\mathbf{v}_1||}, \frac{U\mathbf{v}_2}{||U\mathbf{v}_2||}, \frac{U\mathbf{v}_1 \times U\mathbf{v}_2}{||U\mathbf{v}_1||||U\mathbf{v}_2||}\right)\,, \tag{17}$$

and

$$V = \left(\mathbf{v}_1, \mathbf{v}_2, \mp\mathbf{n}^*_{HP}\right)\,. \tag{18}$$

Finally, using simple matrix algebra, we can find $R = VM^T$ ($V$ and $M$ are unitary matrices and they yield a proper rotation matrix).

## TRANSFORMATION ENERGY

To determine if a transformation mechanism and its corresponding orientation relationship are energetically favorable, we computed the energy gained by austenite atoms from transforming into martensite within an austenite matrix. In particular we considered a martensite plate of dimensions $l \times w \times t$ composed of $n$ atoms where $l \gg t$ and $w \gg t$ (see Fig. 3). In its initial austenite (FCC) state, the total energy of the plate is:

$$E_\gamma = ne_\gamma \tag{19}$$

where $n$ is the number of atoms in the plate and $e_\gamma$ is the energy per austenite atom. In the final martensite state, its energy is given by:

$$E_\alpha = ne_\alpha + 2lwE_{lw} + 2ltE_{lt} + 2wtE_{wt} \tag{20}$$

Where $E_{lw}, E_{lt}, E_{wt}$ are the surface energies per unit area for each face of the plate. Since $lw \gg lt$ and $lw \gg wt$ we can write the equation in terms of the plate's area $A = lw$.

$$E_\alpha = ne_\alpha + 2AE_A \tag{21}$$

Note that we consider the martensite atoms to be strained so the interface A is coherent, therefore $e_\alpha$ is different for each transformation mechanism and OR. Finally, the energy difference per atom is given by the following equation:

$$\frac{\Delta E}{n} = \Delta e + 2\frac{A}{n}E_A \tag{22}$$

Where $\Delta E = E_\alpha - E_\gamma$ and $\Delta e = e_\alpha - e_\gamma$. This expression can be rewritten as a function of the plate's thickness $t$:

$$\frac{\Delta E}{n} = \Delta e + 2\frac{V}{n}\frac{A}{V}E_A \tag{23}$$

$$\frac{\Delta E}{n} = \Delta e + 2v_\gamma\frac{E_A}{t} \tag{24}$$

Where $V = lwt$ is the volume of the plate in its austenite state and $v_\gamma = \frac{V}{n}$ is the specific volume of austenite.

In order to obtain the interface energy $E_A$ and $e_\gamma$, $e_\alpha$, we ran spin-polarized density functional theory (DFT) calculations in the local density approximation with the projector augmented wave method [3] as implemented in VASP [4].

First, we found the total energy for pure austenite to obtain $e_\gamma$. Secondly, for each mechanism, to obtain $e_\alpha$, we found the energy of pure martensite under the same strain conditions as in the plate. Thirdly, we computed the total energy $E_{\mathrm{slab}}$ of slabs composed of strained martensite sandwiched between two layers of austenite; examples are shown on Fig. 5. In these structures, the area $A$ is infinite because of the periodic boundary condition and the thickness is finite and known. To obtain the interface energy per unit area $E_A$, we used the following equation:

$$E_A = \frac{E_{\mathrm{slab}} - n_\gamma e_\gamma - n_\alpha e_\alpha}{2A_{\mathrm{slab}}} \tag{25}$$

With this information, we computed equation (24) for our proposed mechanism (New), for the Kurdjumov-Sach mechanism (K-S) [5] [6] and for the Bain mechanism (Bain). The results are shown on Fig. 4. It is clear from the figure that, for any realistic plate thicker than 1 nm, our proposed mechanism is the most energetically favorable.

In Fig. 3 of the paper, using the same DFT approach, we directly computed the change in energy per transformed atom $\frac{\Delta E}{n_b}$ along the transformation at a specific thickness of 1.8 nm. To do so, we used the following equation:

$$\frac{\Delta E^i}{n} = \frac{E^i_{\mathrm{slab}} - ne_\gamma}{n_{\mathrm{trans}}} \tag{26}$$

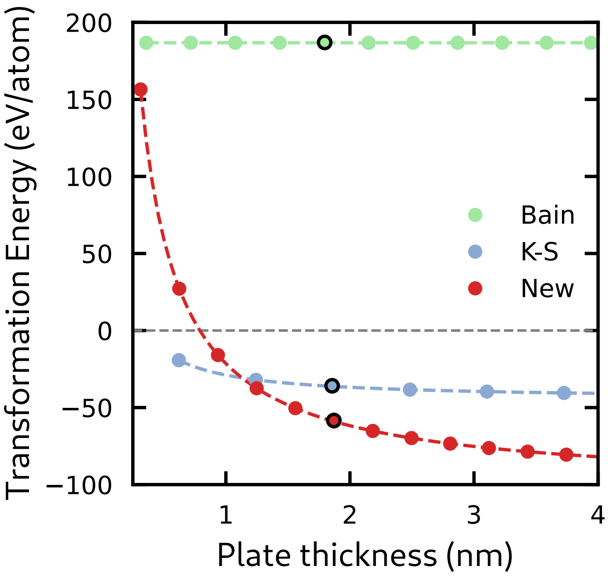


FIG. 4. Energy difference between atoms in the austenite and martensite states within an austenite matrix as a function of the plate's thickness for three transformation mechanisms. Points that are outlined correspond to the transformation shown in Fig. 3 of this paper.

Where $n_{\text{trans}}$ is the number of atoms that transform from austenite to martensite such that $n = n_\gamma + n_{\text{trans}}$ and $i$ is the step along the transformation. For example, $E^0_{\text{slab}} = ne_\gamma$ is the energy of a pure supercell of austenite where $\frac{\Delta E^0}{n_b} = 0$. The exact structures that were used for calculations of the final transformed state in Fig. 3 of the paper are presented on Fig. 5 they also correspond to the outlined points in Fig. 4


[1] F. Therrien, P. Graf, and V. Stevanović, Matching crystal structures atom-to-atom, The Journal of Chemical Physics **152**, 074106 (2020).

[2] V. Stevanović, R. Trottier, C. Musgrave, F. Therrien, A. Holder, and P. Graf, Predicting kinetics of polymorphic transformations from structure mapping and coordination analysis, Phys. Rev. Materials **2** (2018).

[3] P. E. Blöchl, Projector augmented-wave method, Physical review B **50**, 17953 (1994).

[4] G. Kresse and J. Furthmüller, Efficiency of ab-initio total energy calculations for metals and semiconductors using a plane-wave basis set, Computational materials science **6**, 15 (1996).

[5] Z. Nishiyama, *Martensitic transformation* (Elsevier, 2012).

[6] In this case, since the final martensite state is strained to make the interface coherent, this mechanism is exactly equivalent to the Nishiyama shear process.

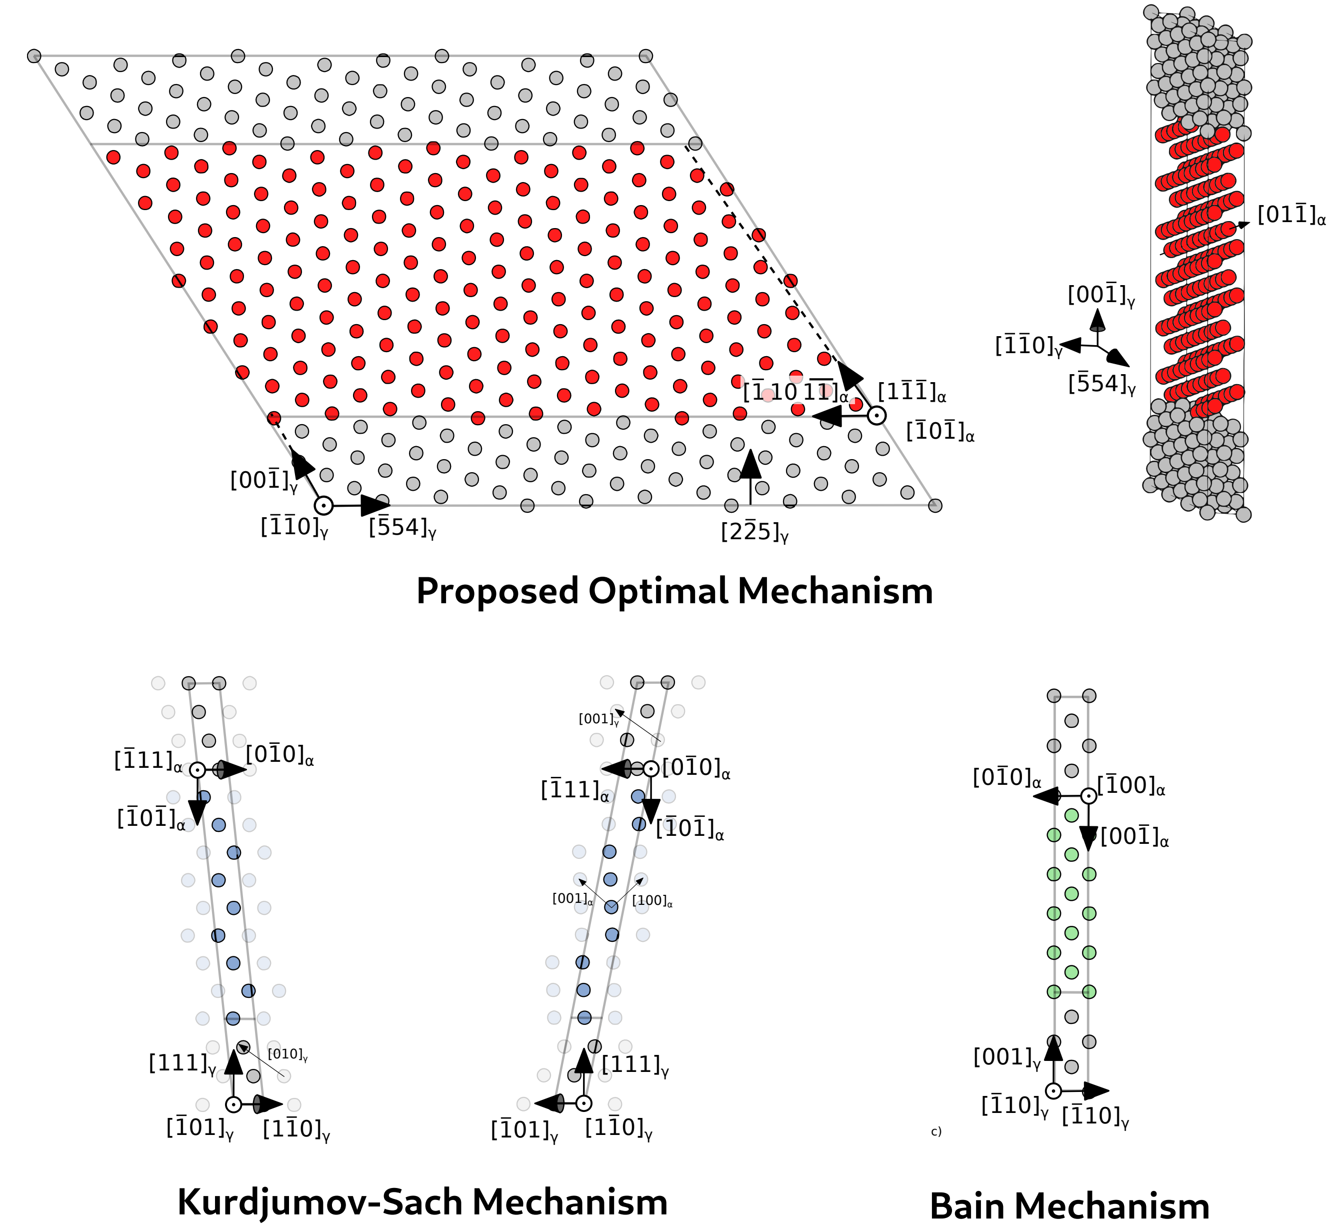


FIG. 5. Crystal structures used to calculate the change in energy per transformed atom in Fig. 3. The colored atoms (red, blue, green) form a strained body centered cubic lattice whereas gray atoms form a face centered cubic lattice.
